# Supplementary material for: Measurement of the CKM angle $\gamma$ from a combination of LHCb results
Source: arXiv:1611.03076 source file (2016-12-21)
Supplement: Supplementary file 3 [file supplementary-app.tex]

\clearpage

\section*{Supplementary material for LHCb-PAPER-2016-032}
\label{sec:Supplementary-App}

This appendix contains supplementary material that will posted
on the public CDS record but will not appear in the PAPER.

\begin{figure}[h!]
  \centering
  \includegraphics[width=0.6\textwidth]{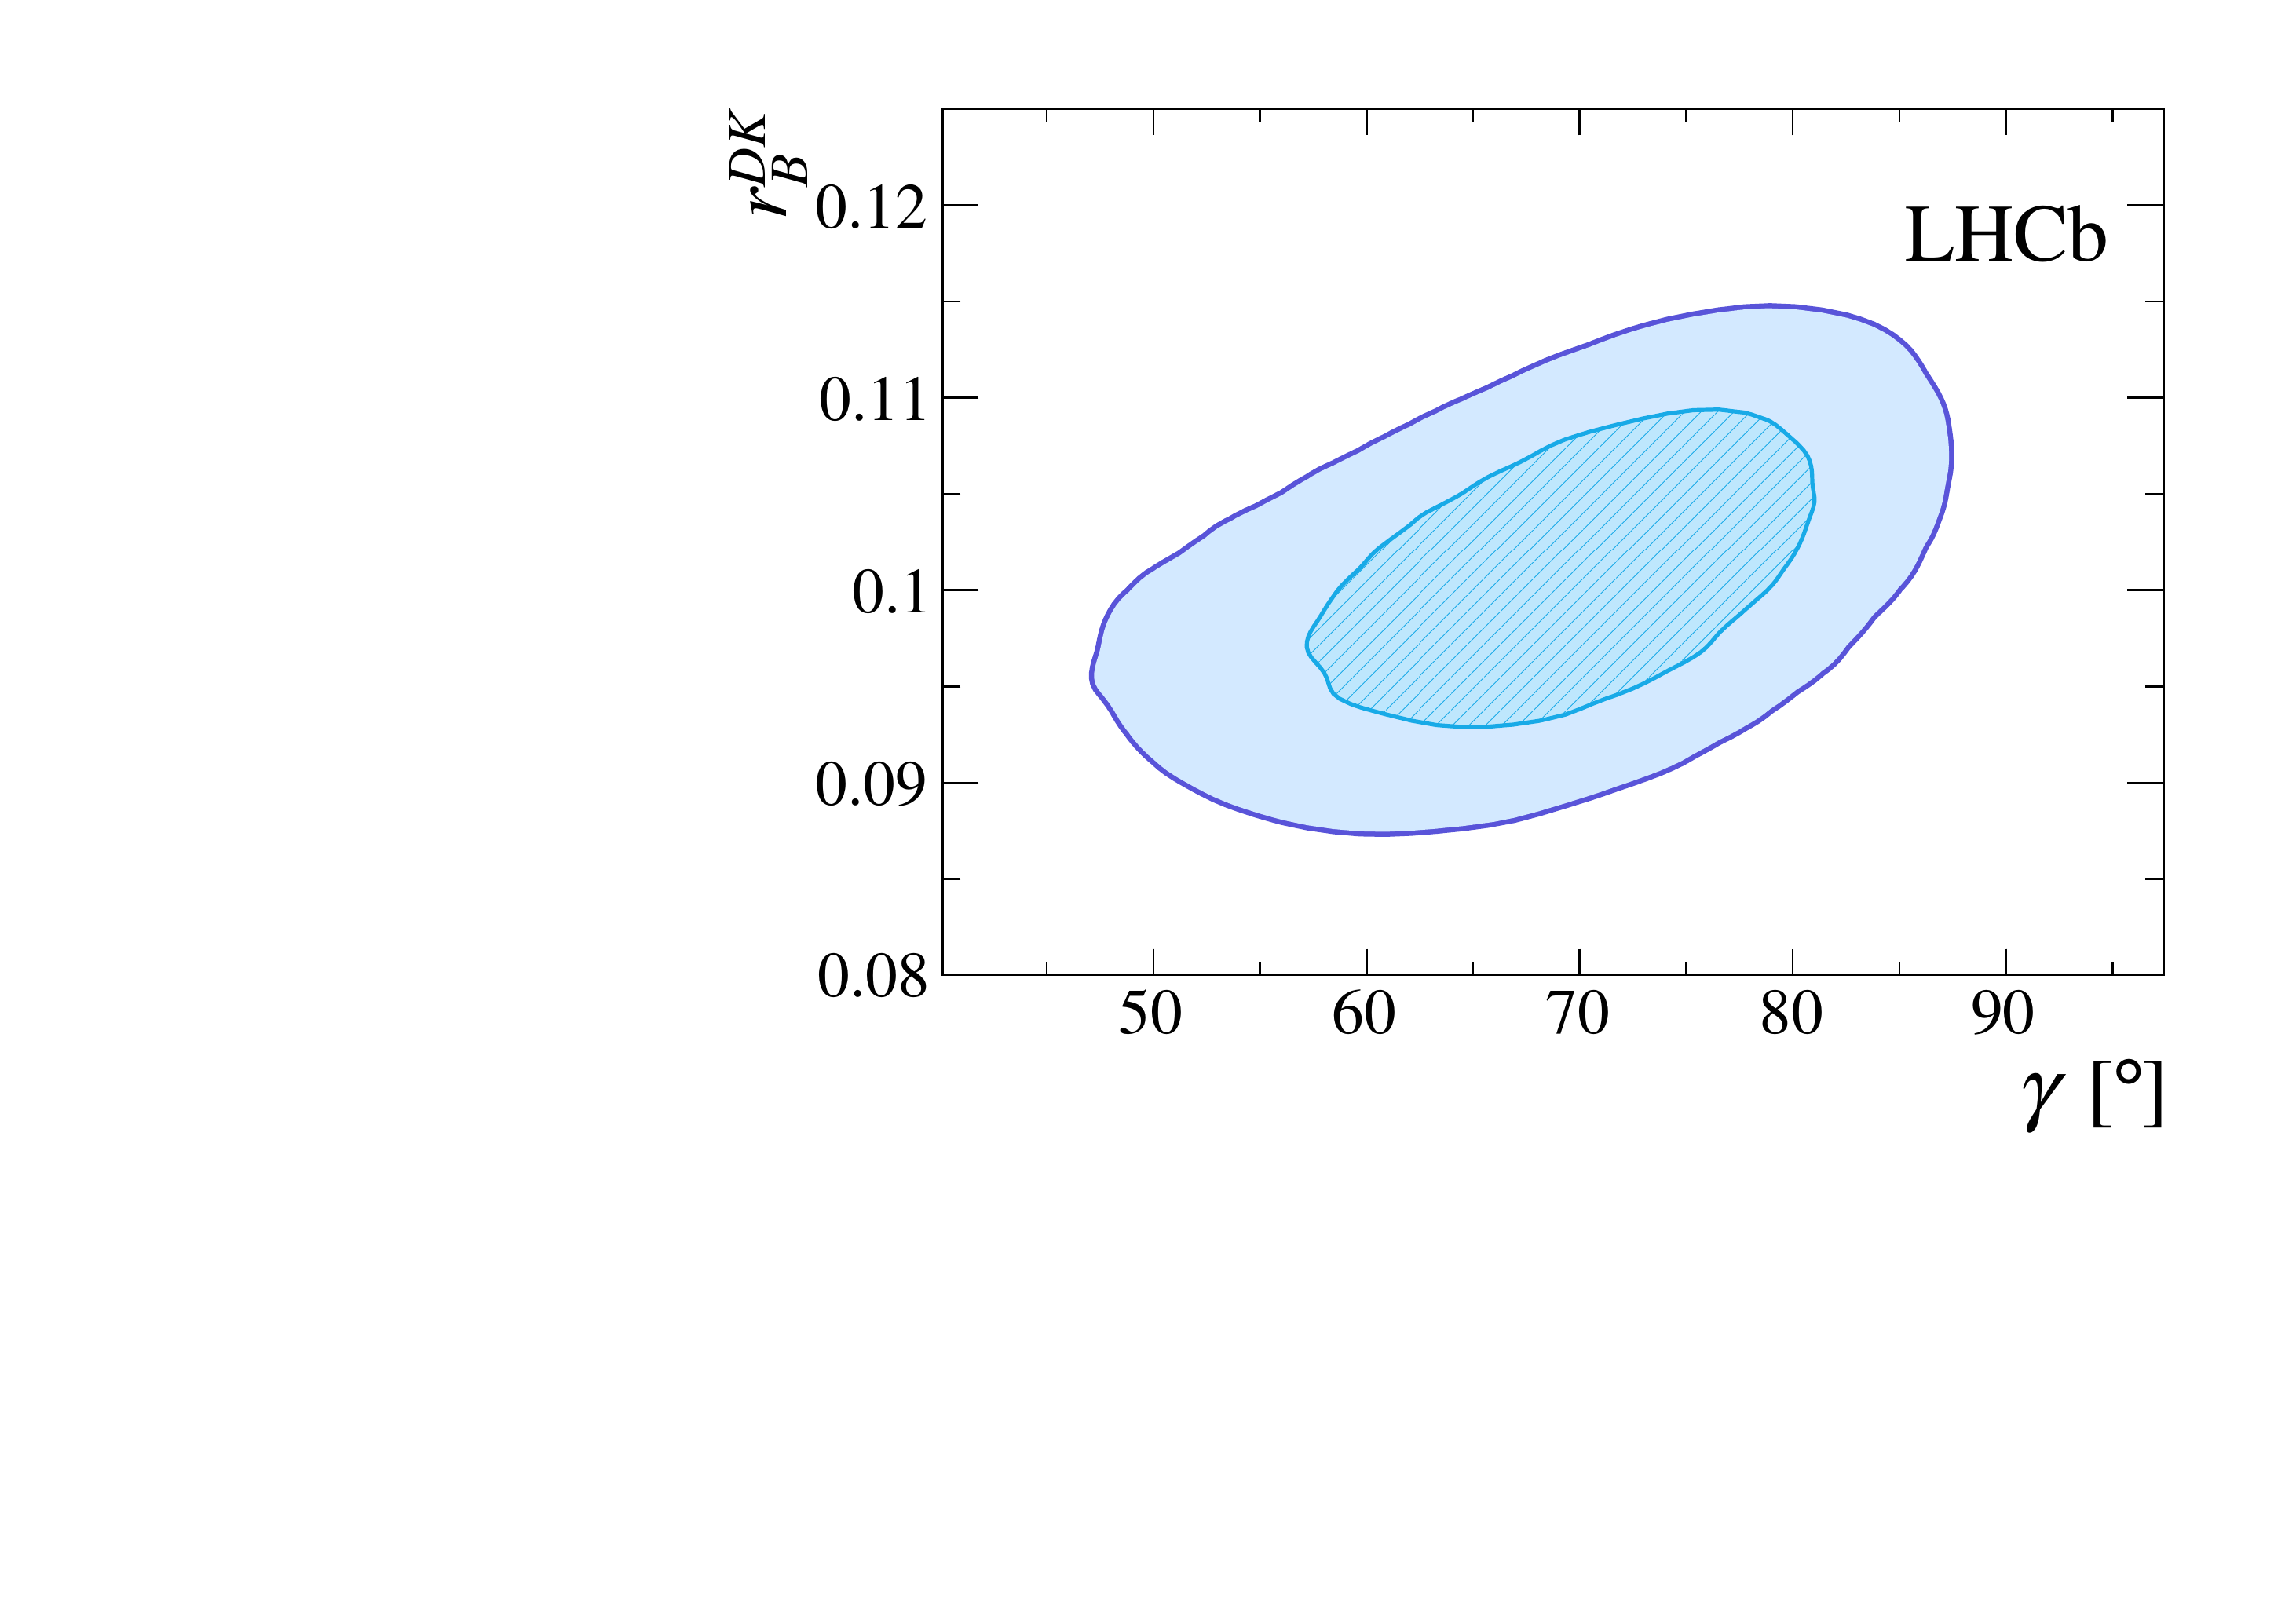}
  \raisebox{0.5\height}{\includegraphics[width=0.3\textwidth]{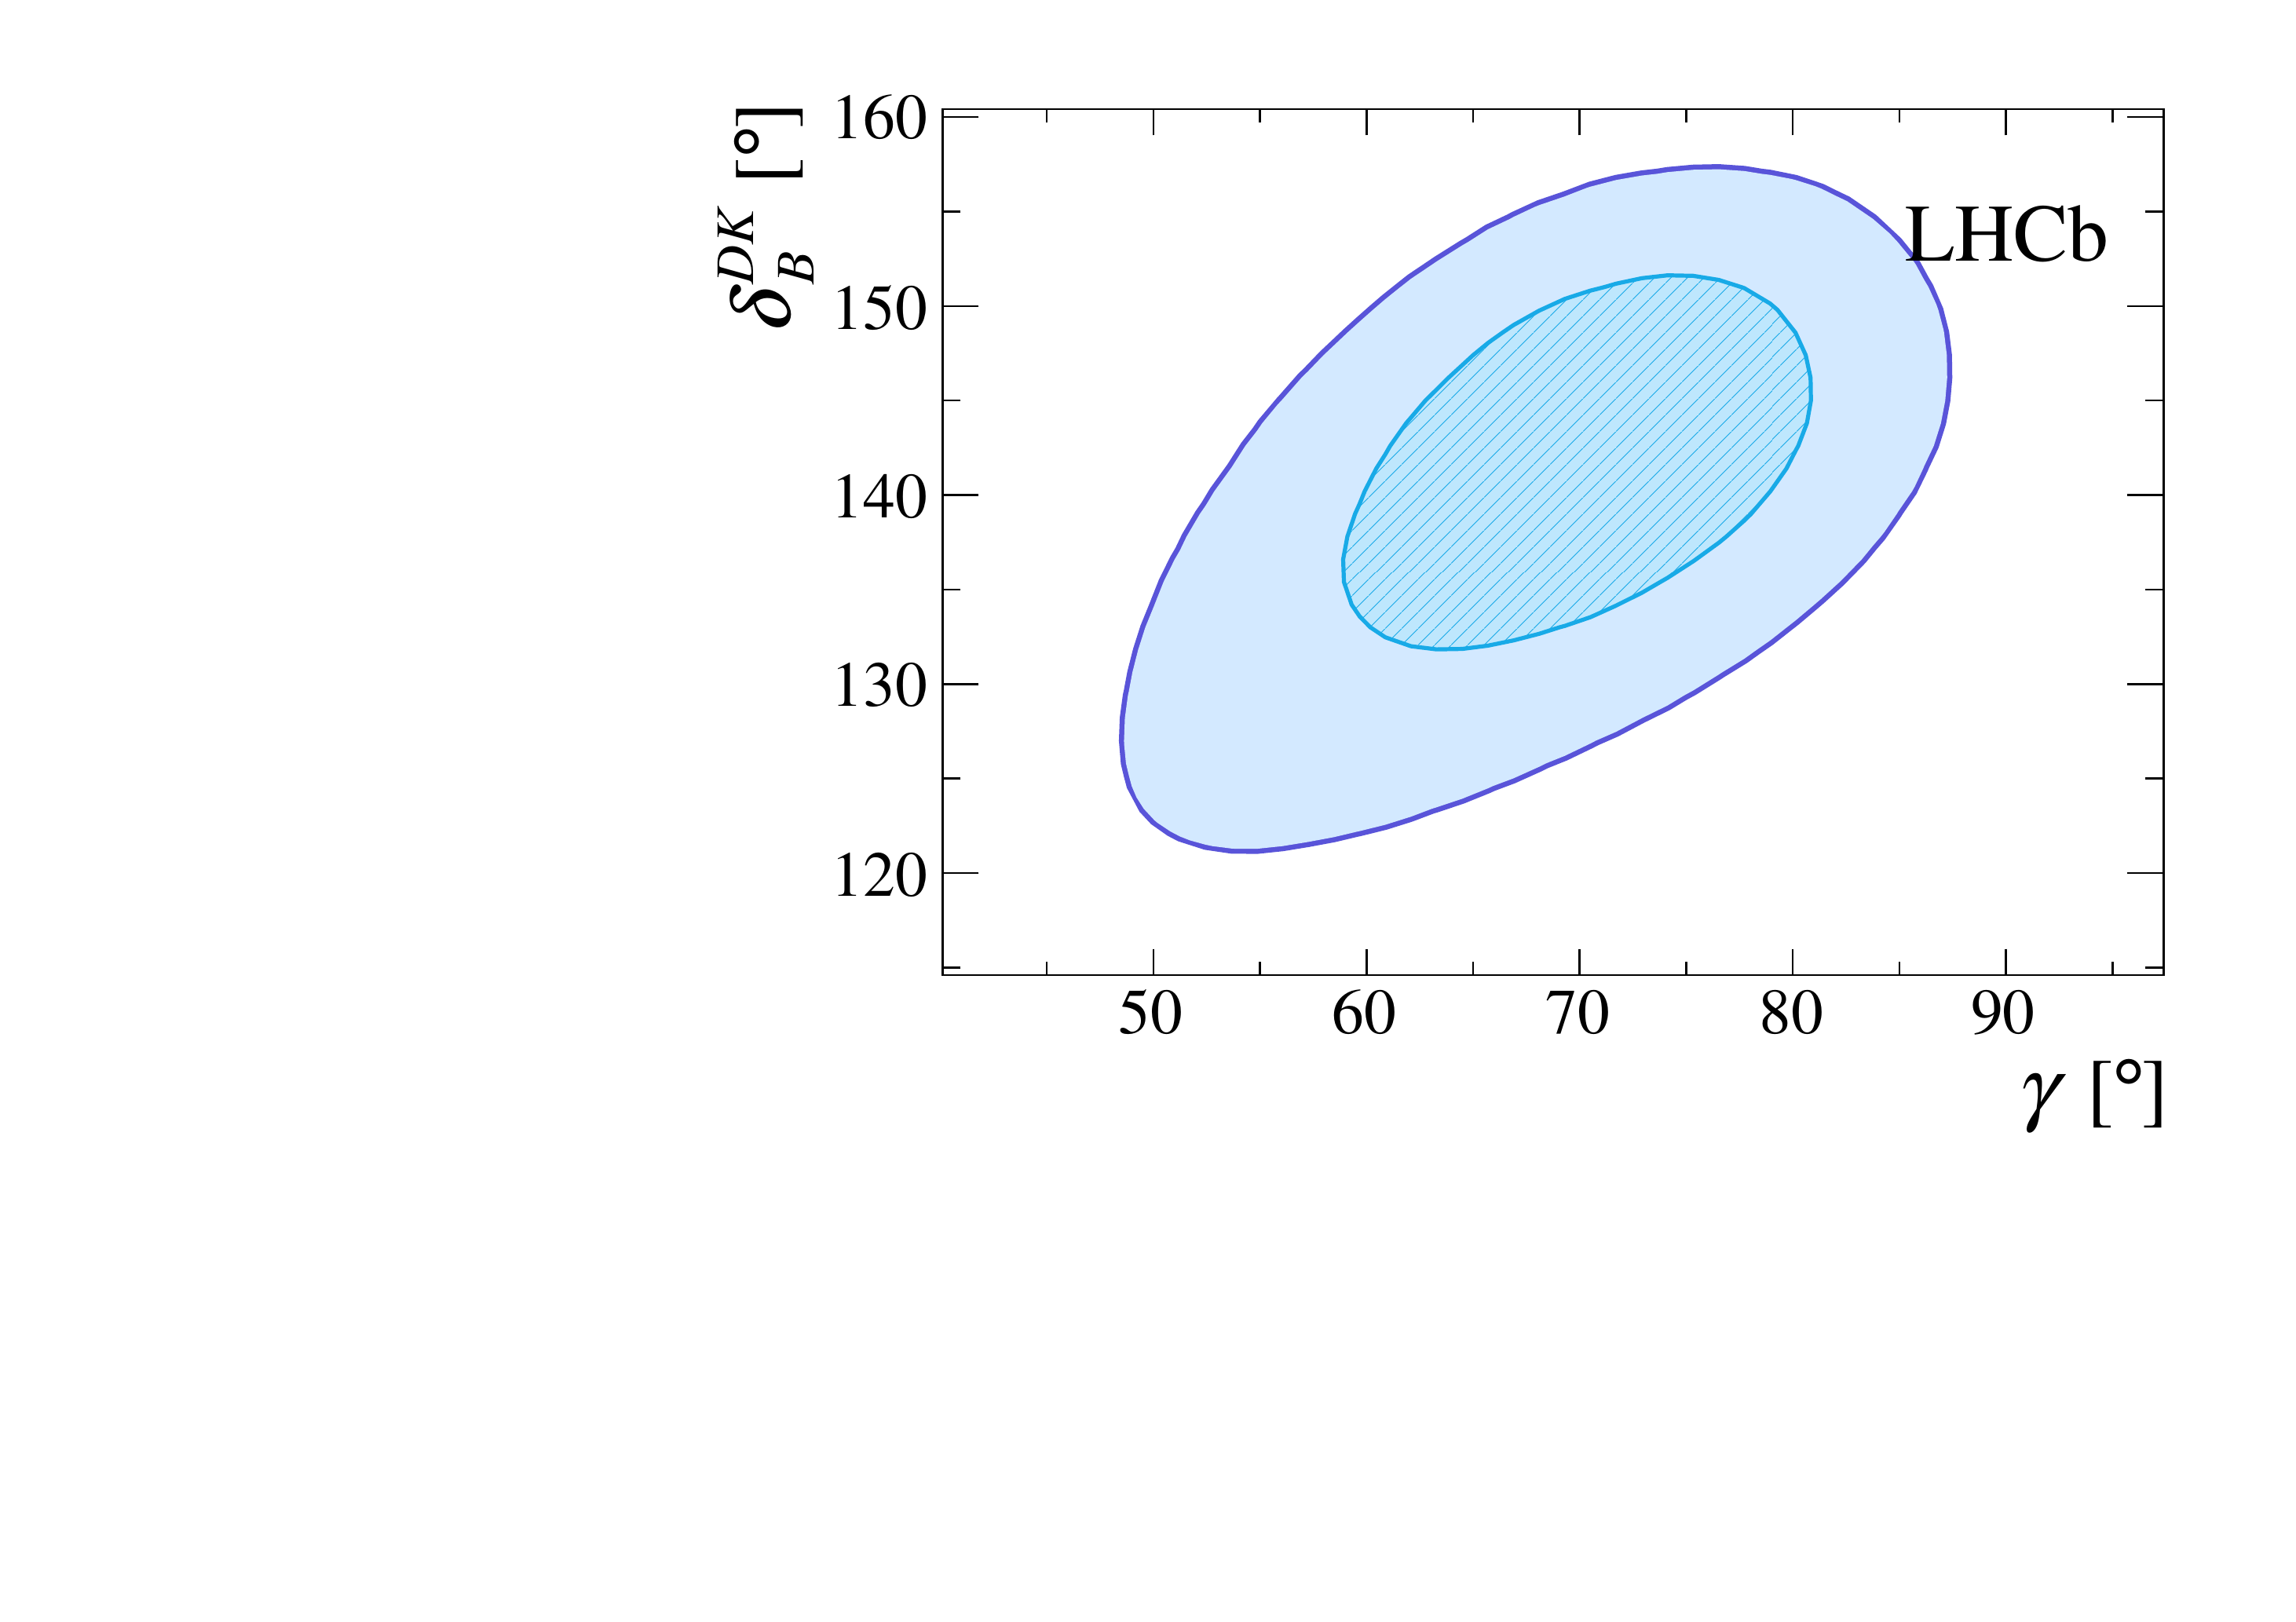}}
  \caption{\omcl plots, using the profile likelihood method, for \DK combinations split by the initial $B$ meson flavour: (orange) \Bs, (yellow) \Bd, (blue) \Bu and (green) the full combination.}
  \label{fig:split_by_b}
\end{figure}

\begin{figure}[h!]
    \centering
    \includegraphics[width=0.6\textwidth]{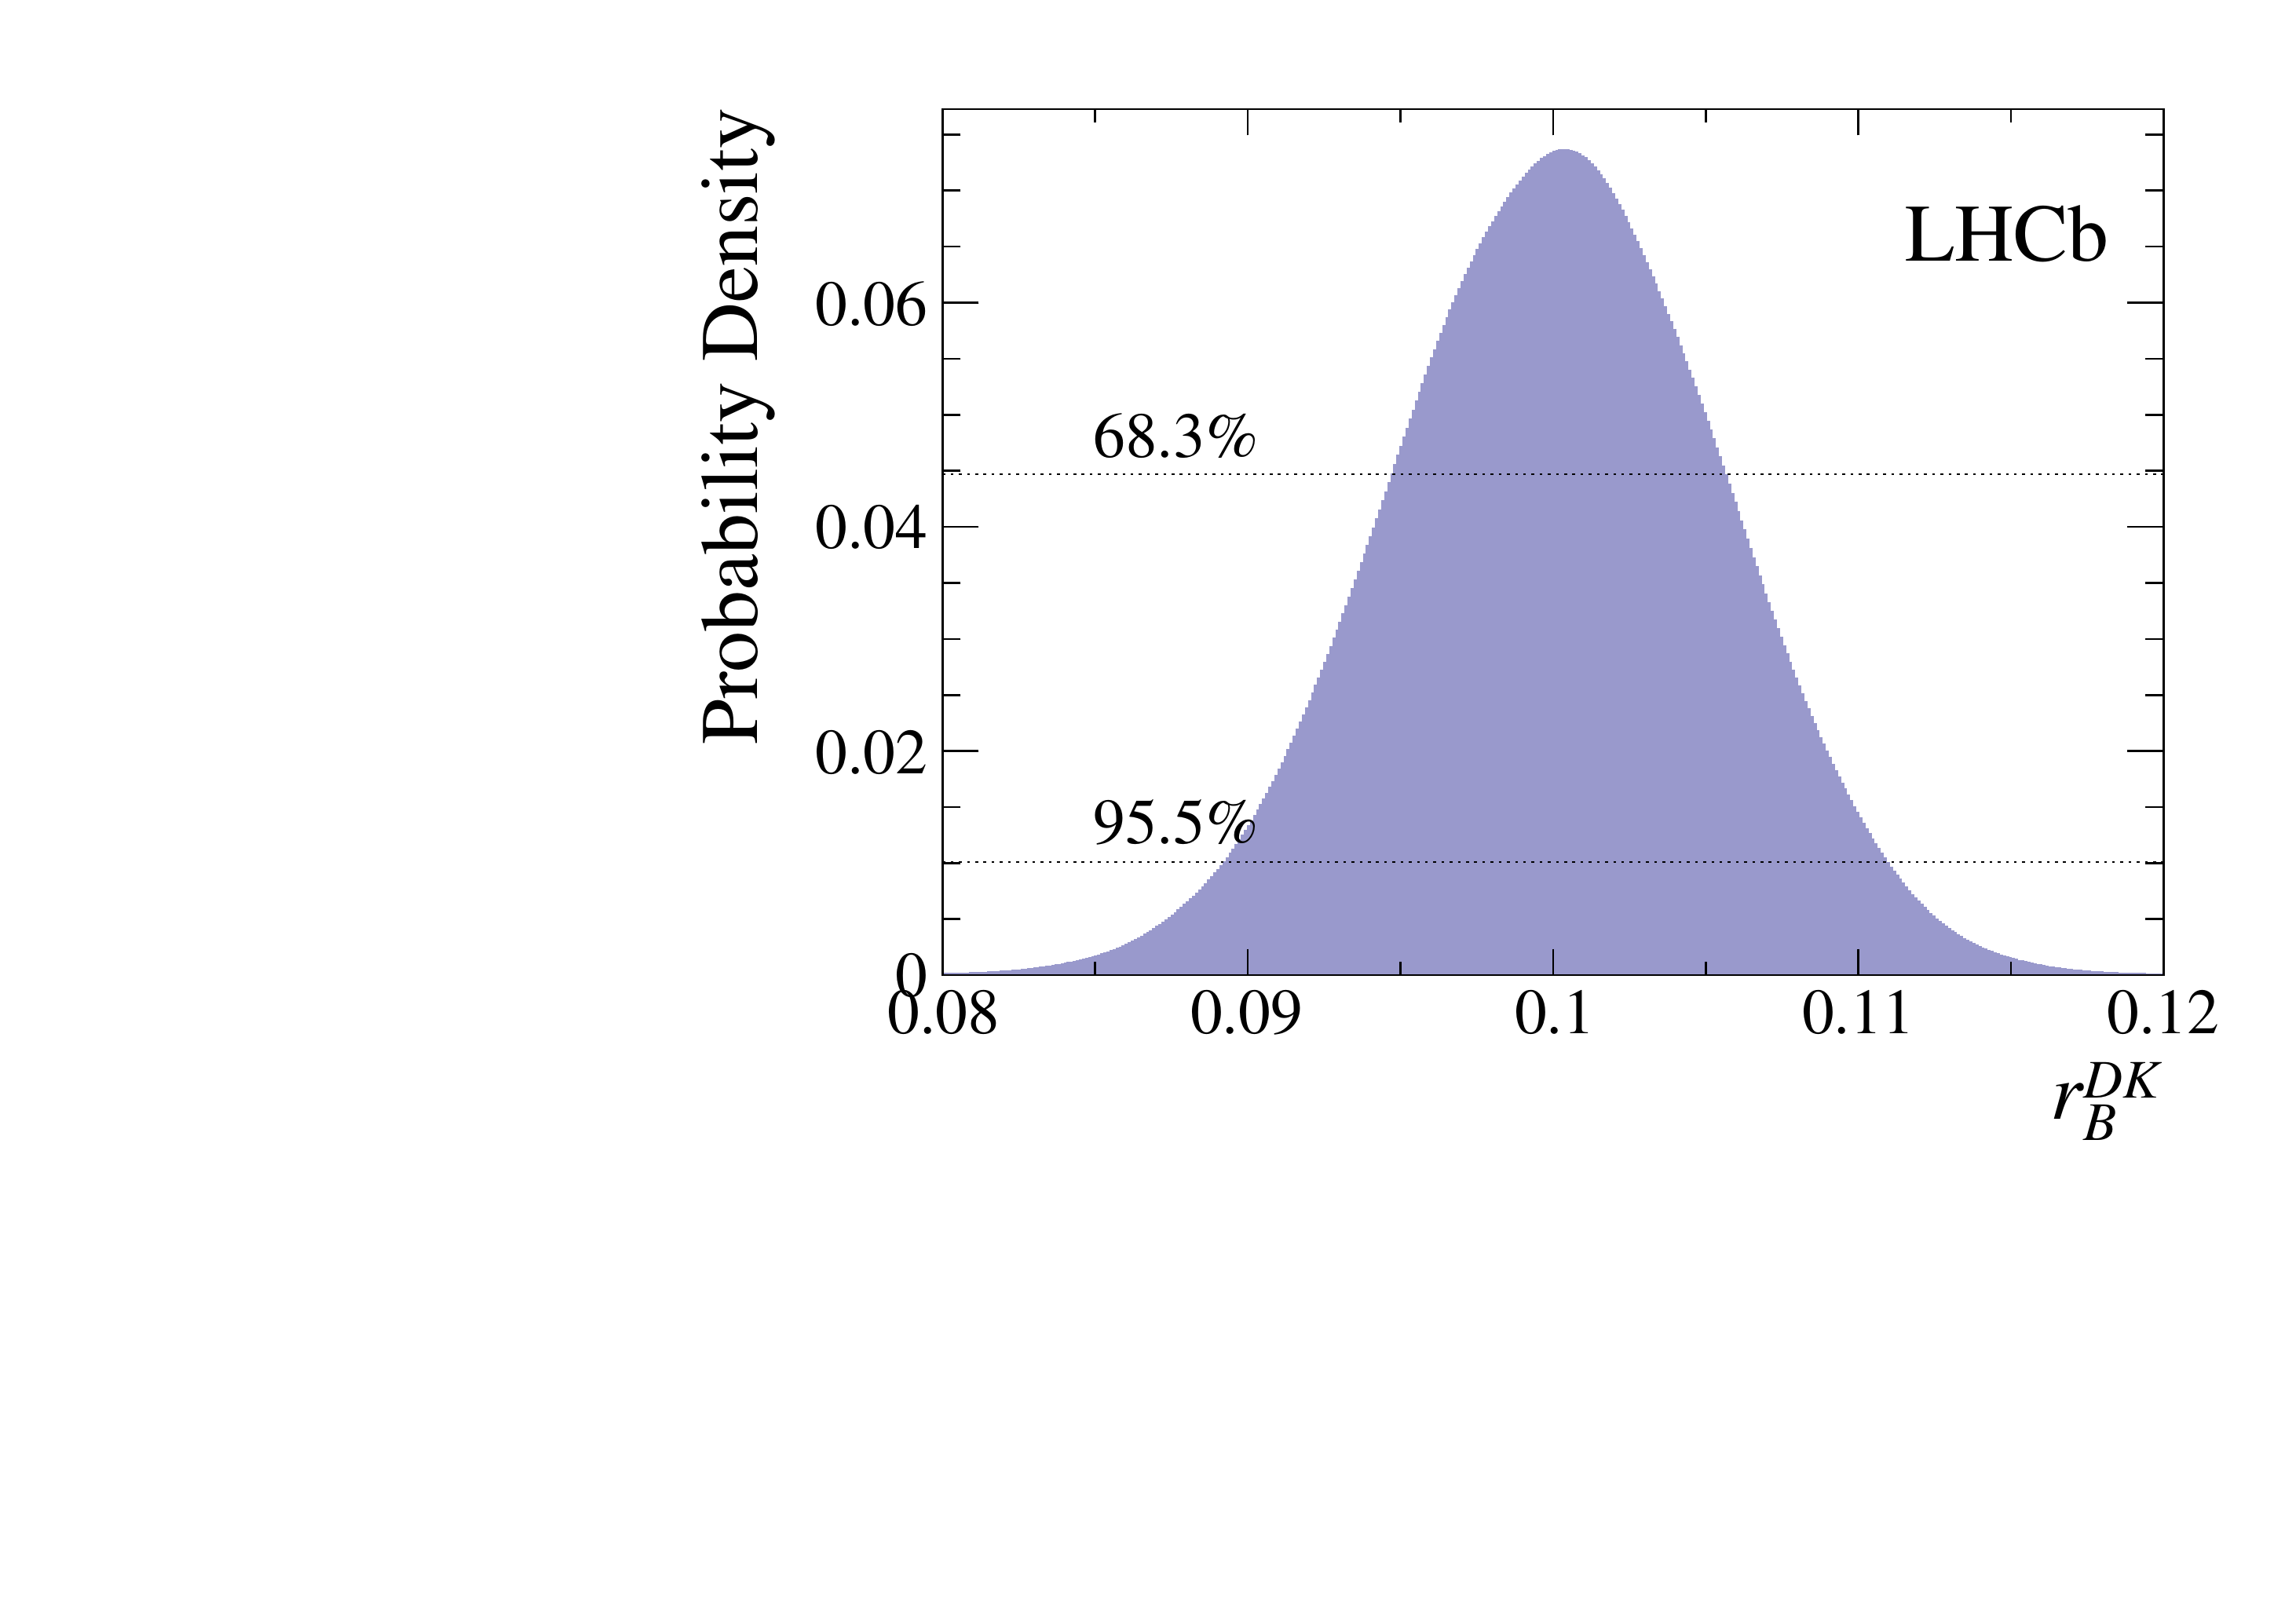}
    \raisebox{0.5\height}{\includegraphics[width=0.3\textwidth]{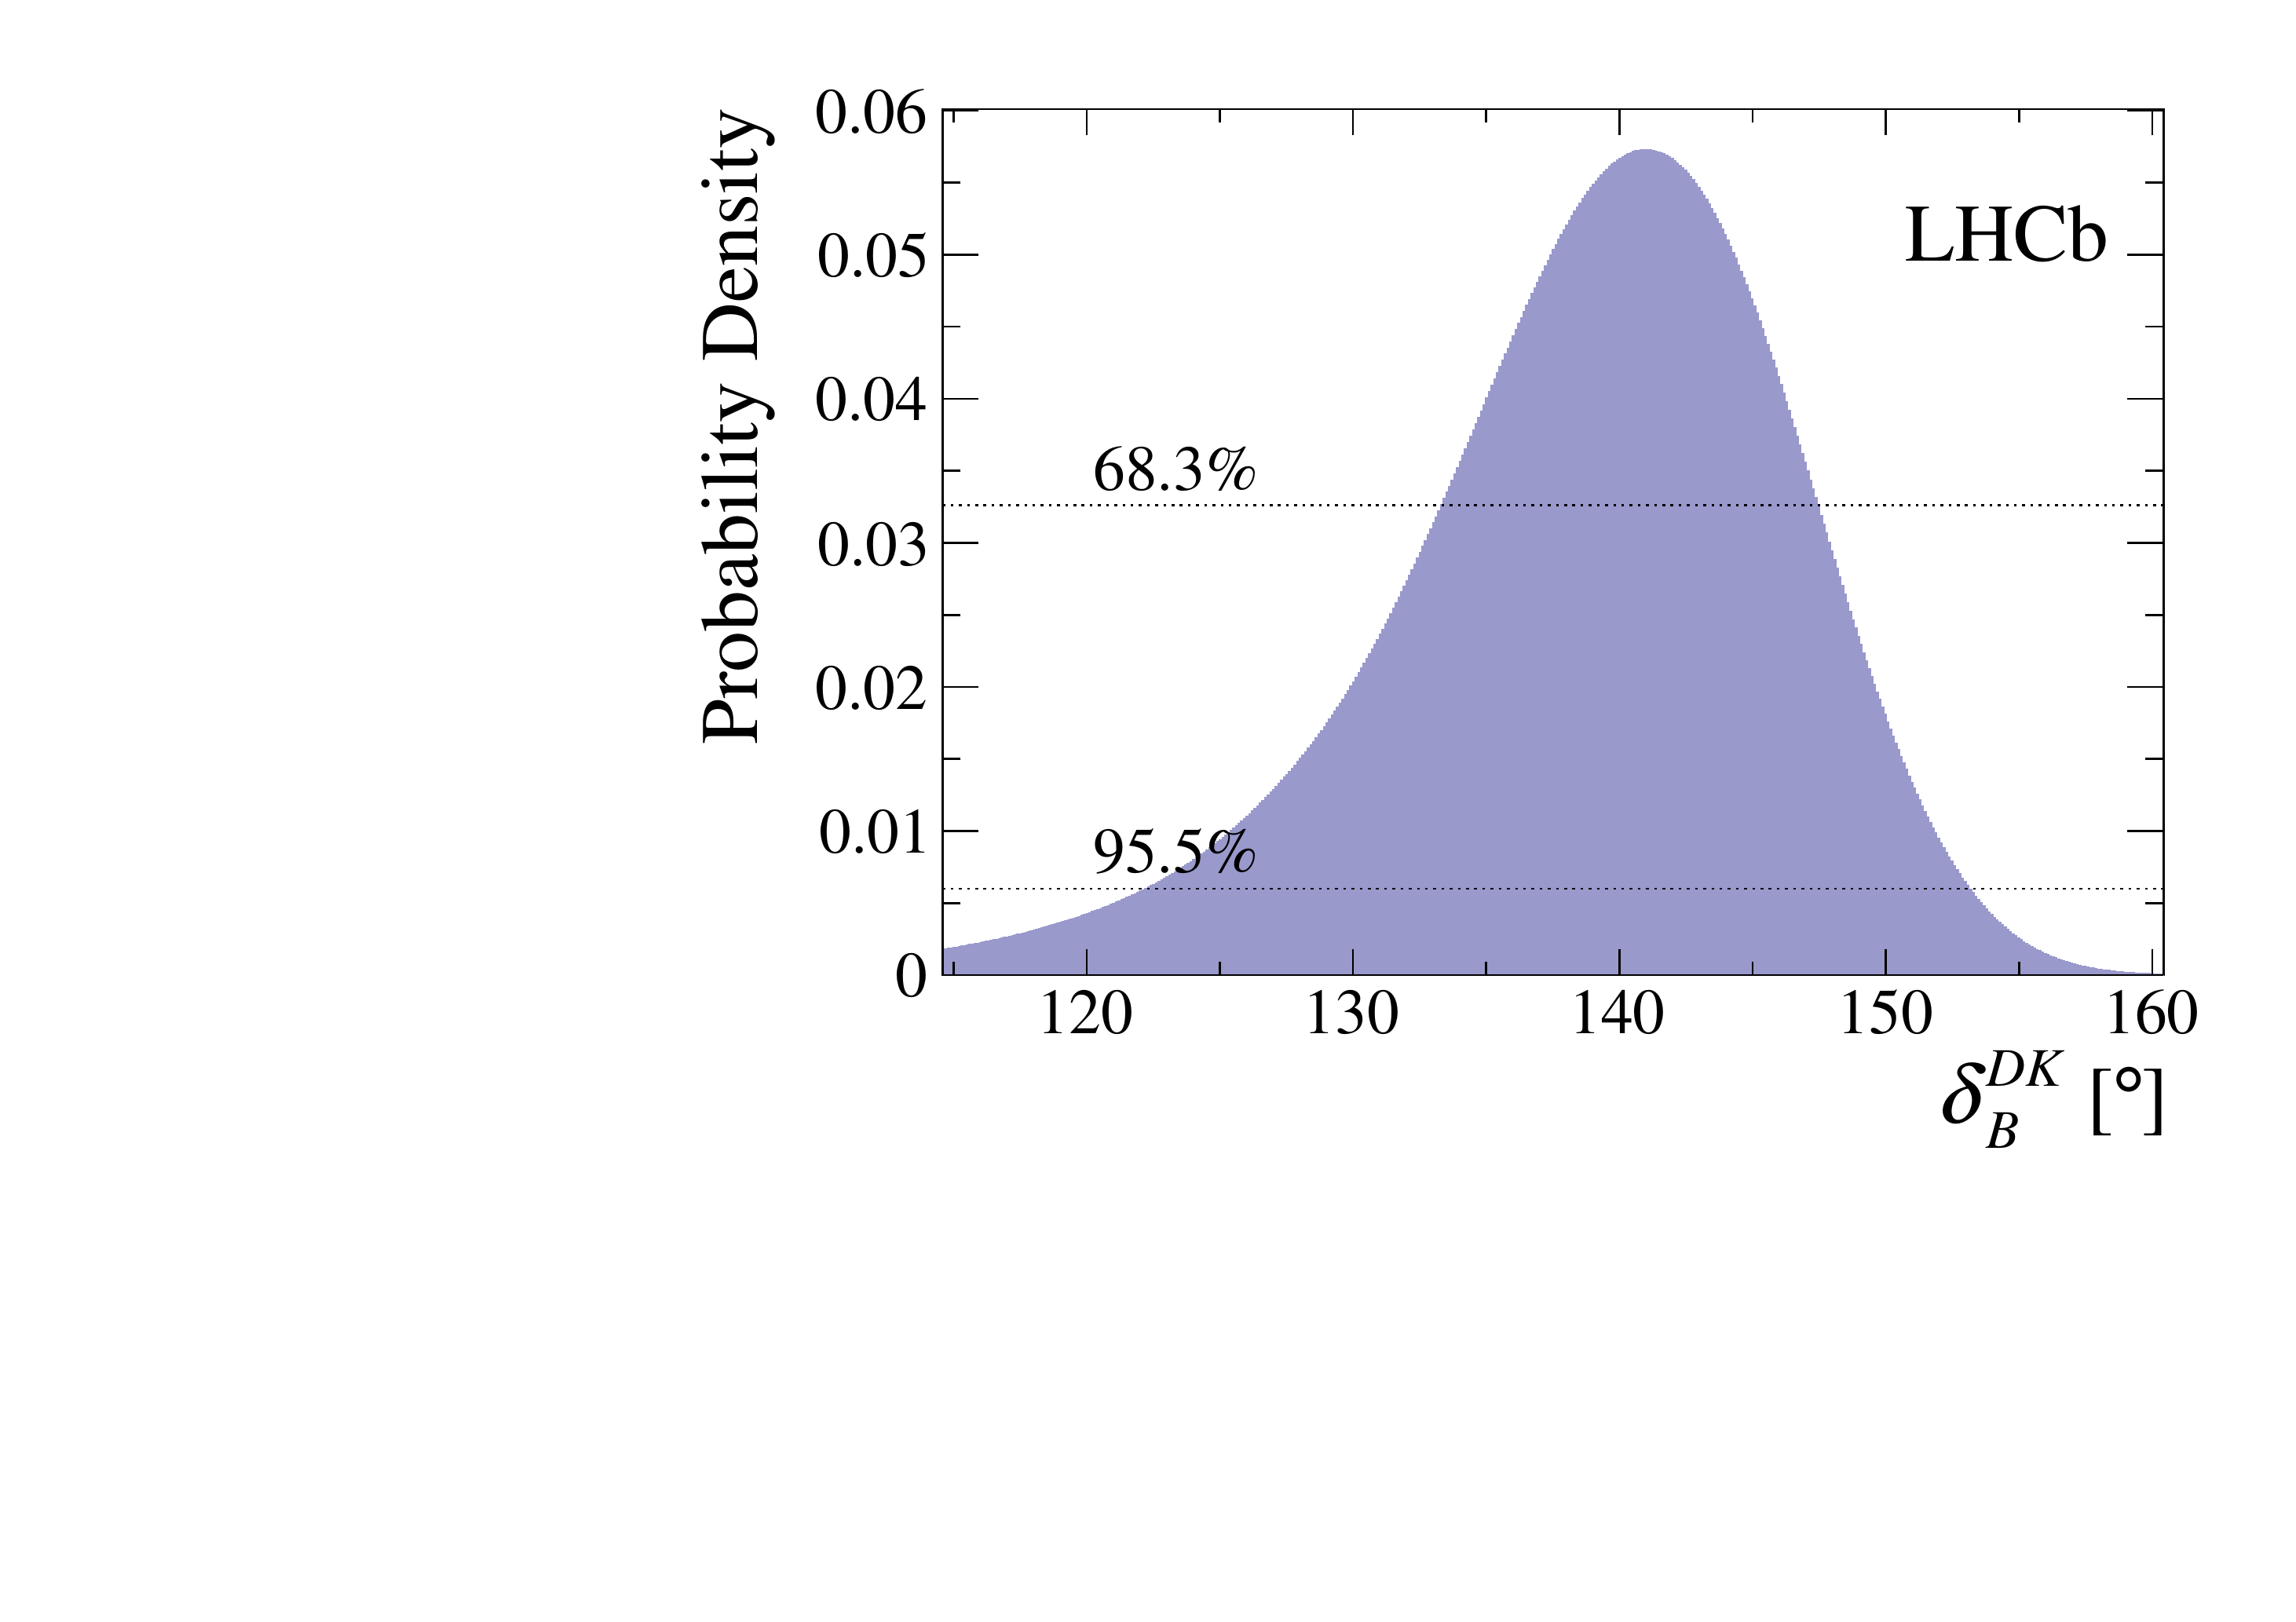}}
    \caption{\omcl plots, using the profile likelihood method, for \DK combinations split by analysis method: (yellow) GGSZ, (orange) GLW/ADS, (blue) others and (green) the full combination.}
    \label{fig:split_by_method}
\end{figure}

\begin{figure}[h!]
  \begin{center}
    \includegraphics[width=0.48\textwidth]{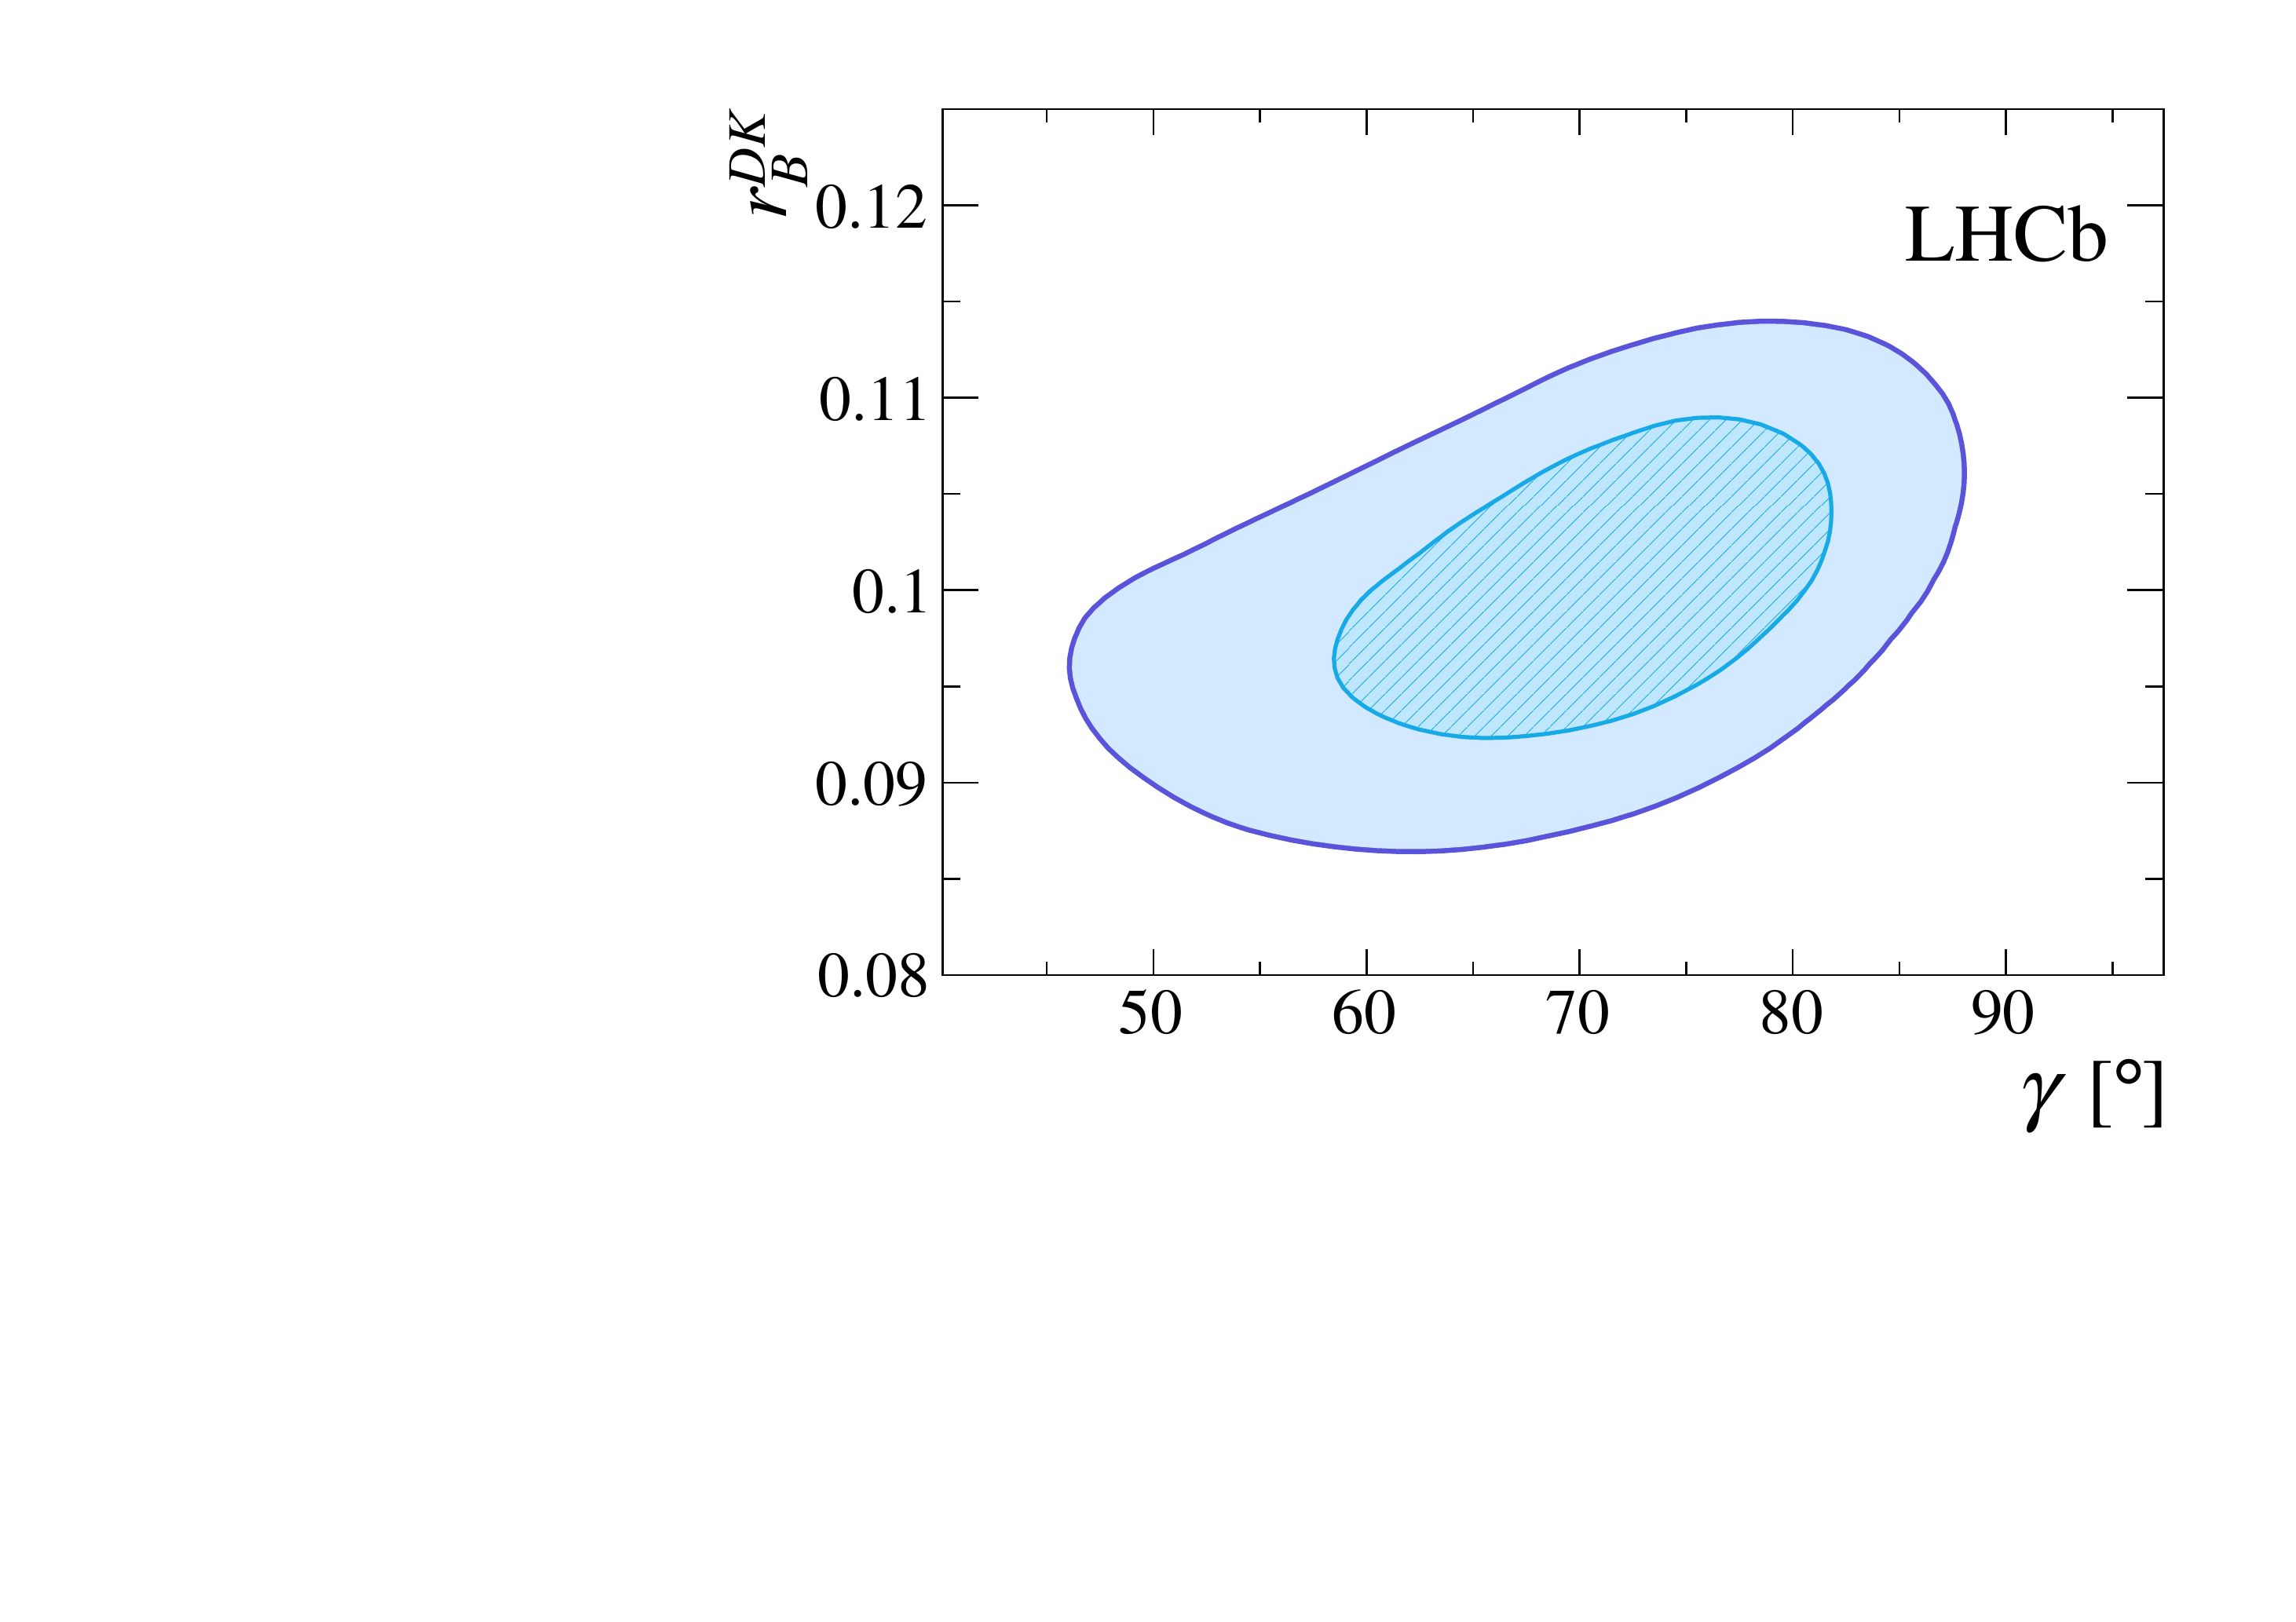}
    \includegraphics[width=0.48\textwidth]{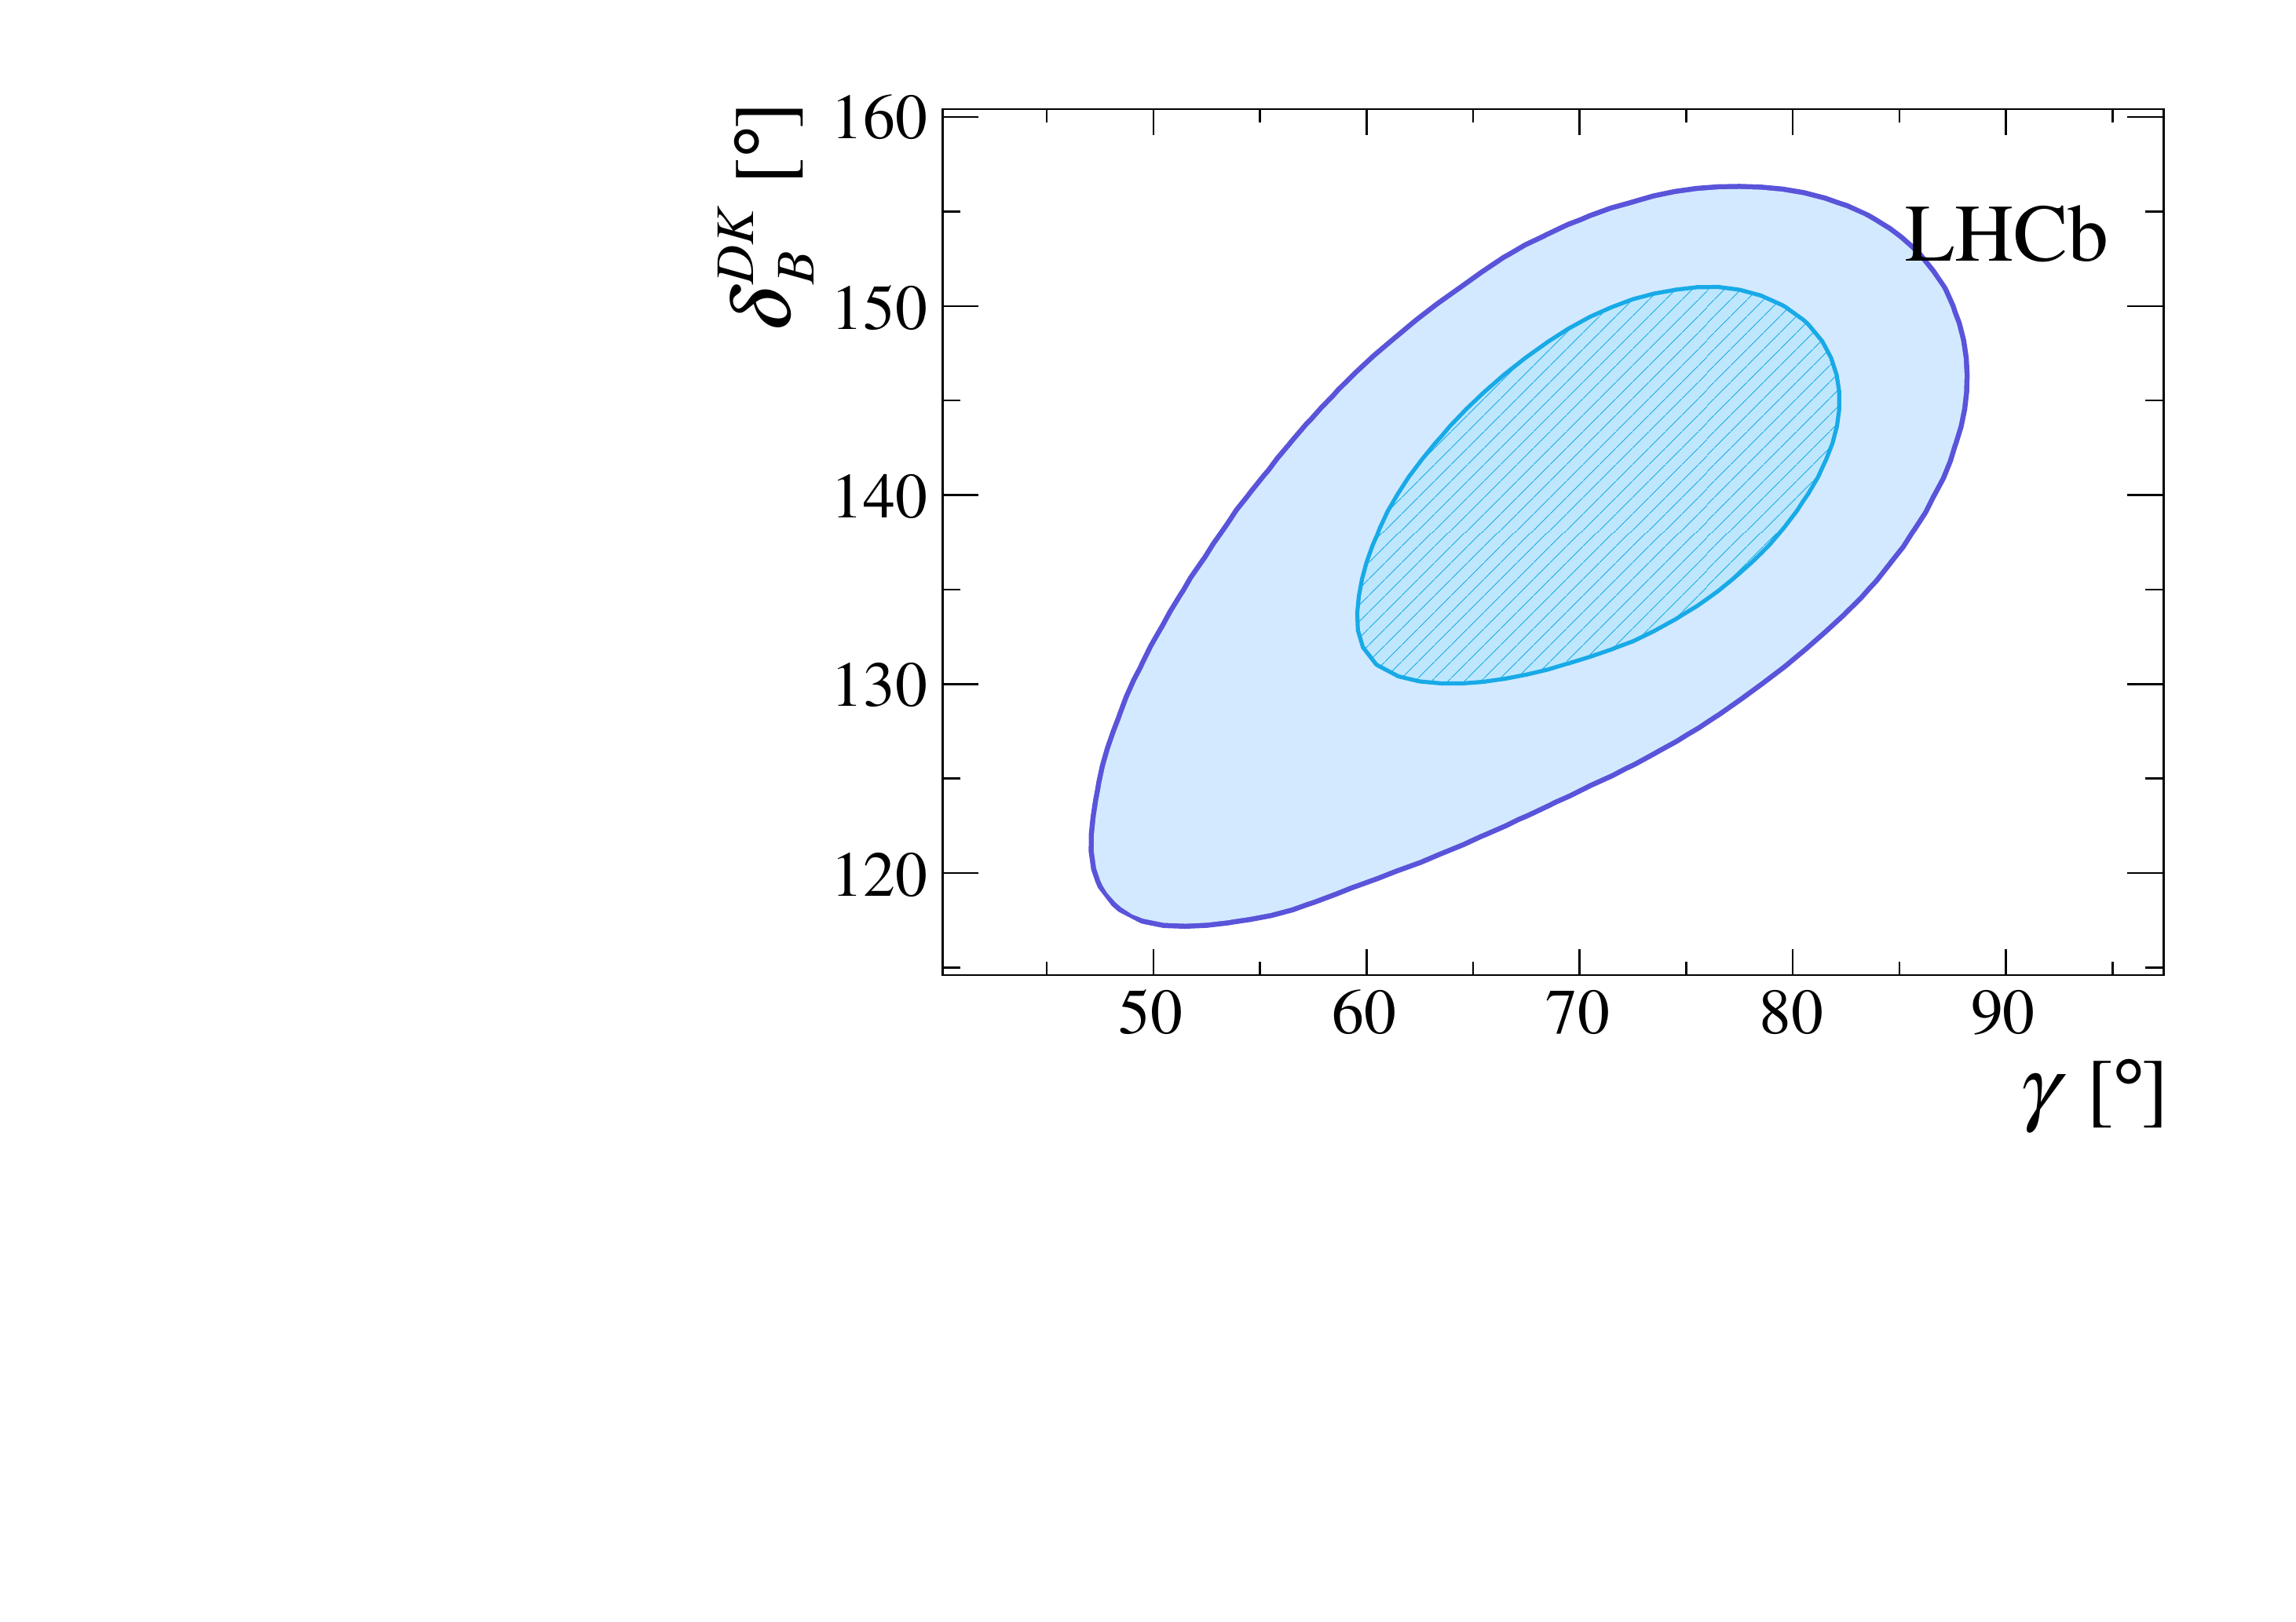} \\
    \includegraphics[width=0.3\textwidth]{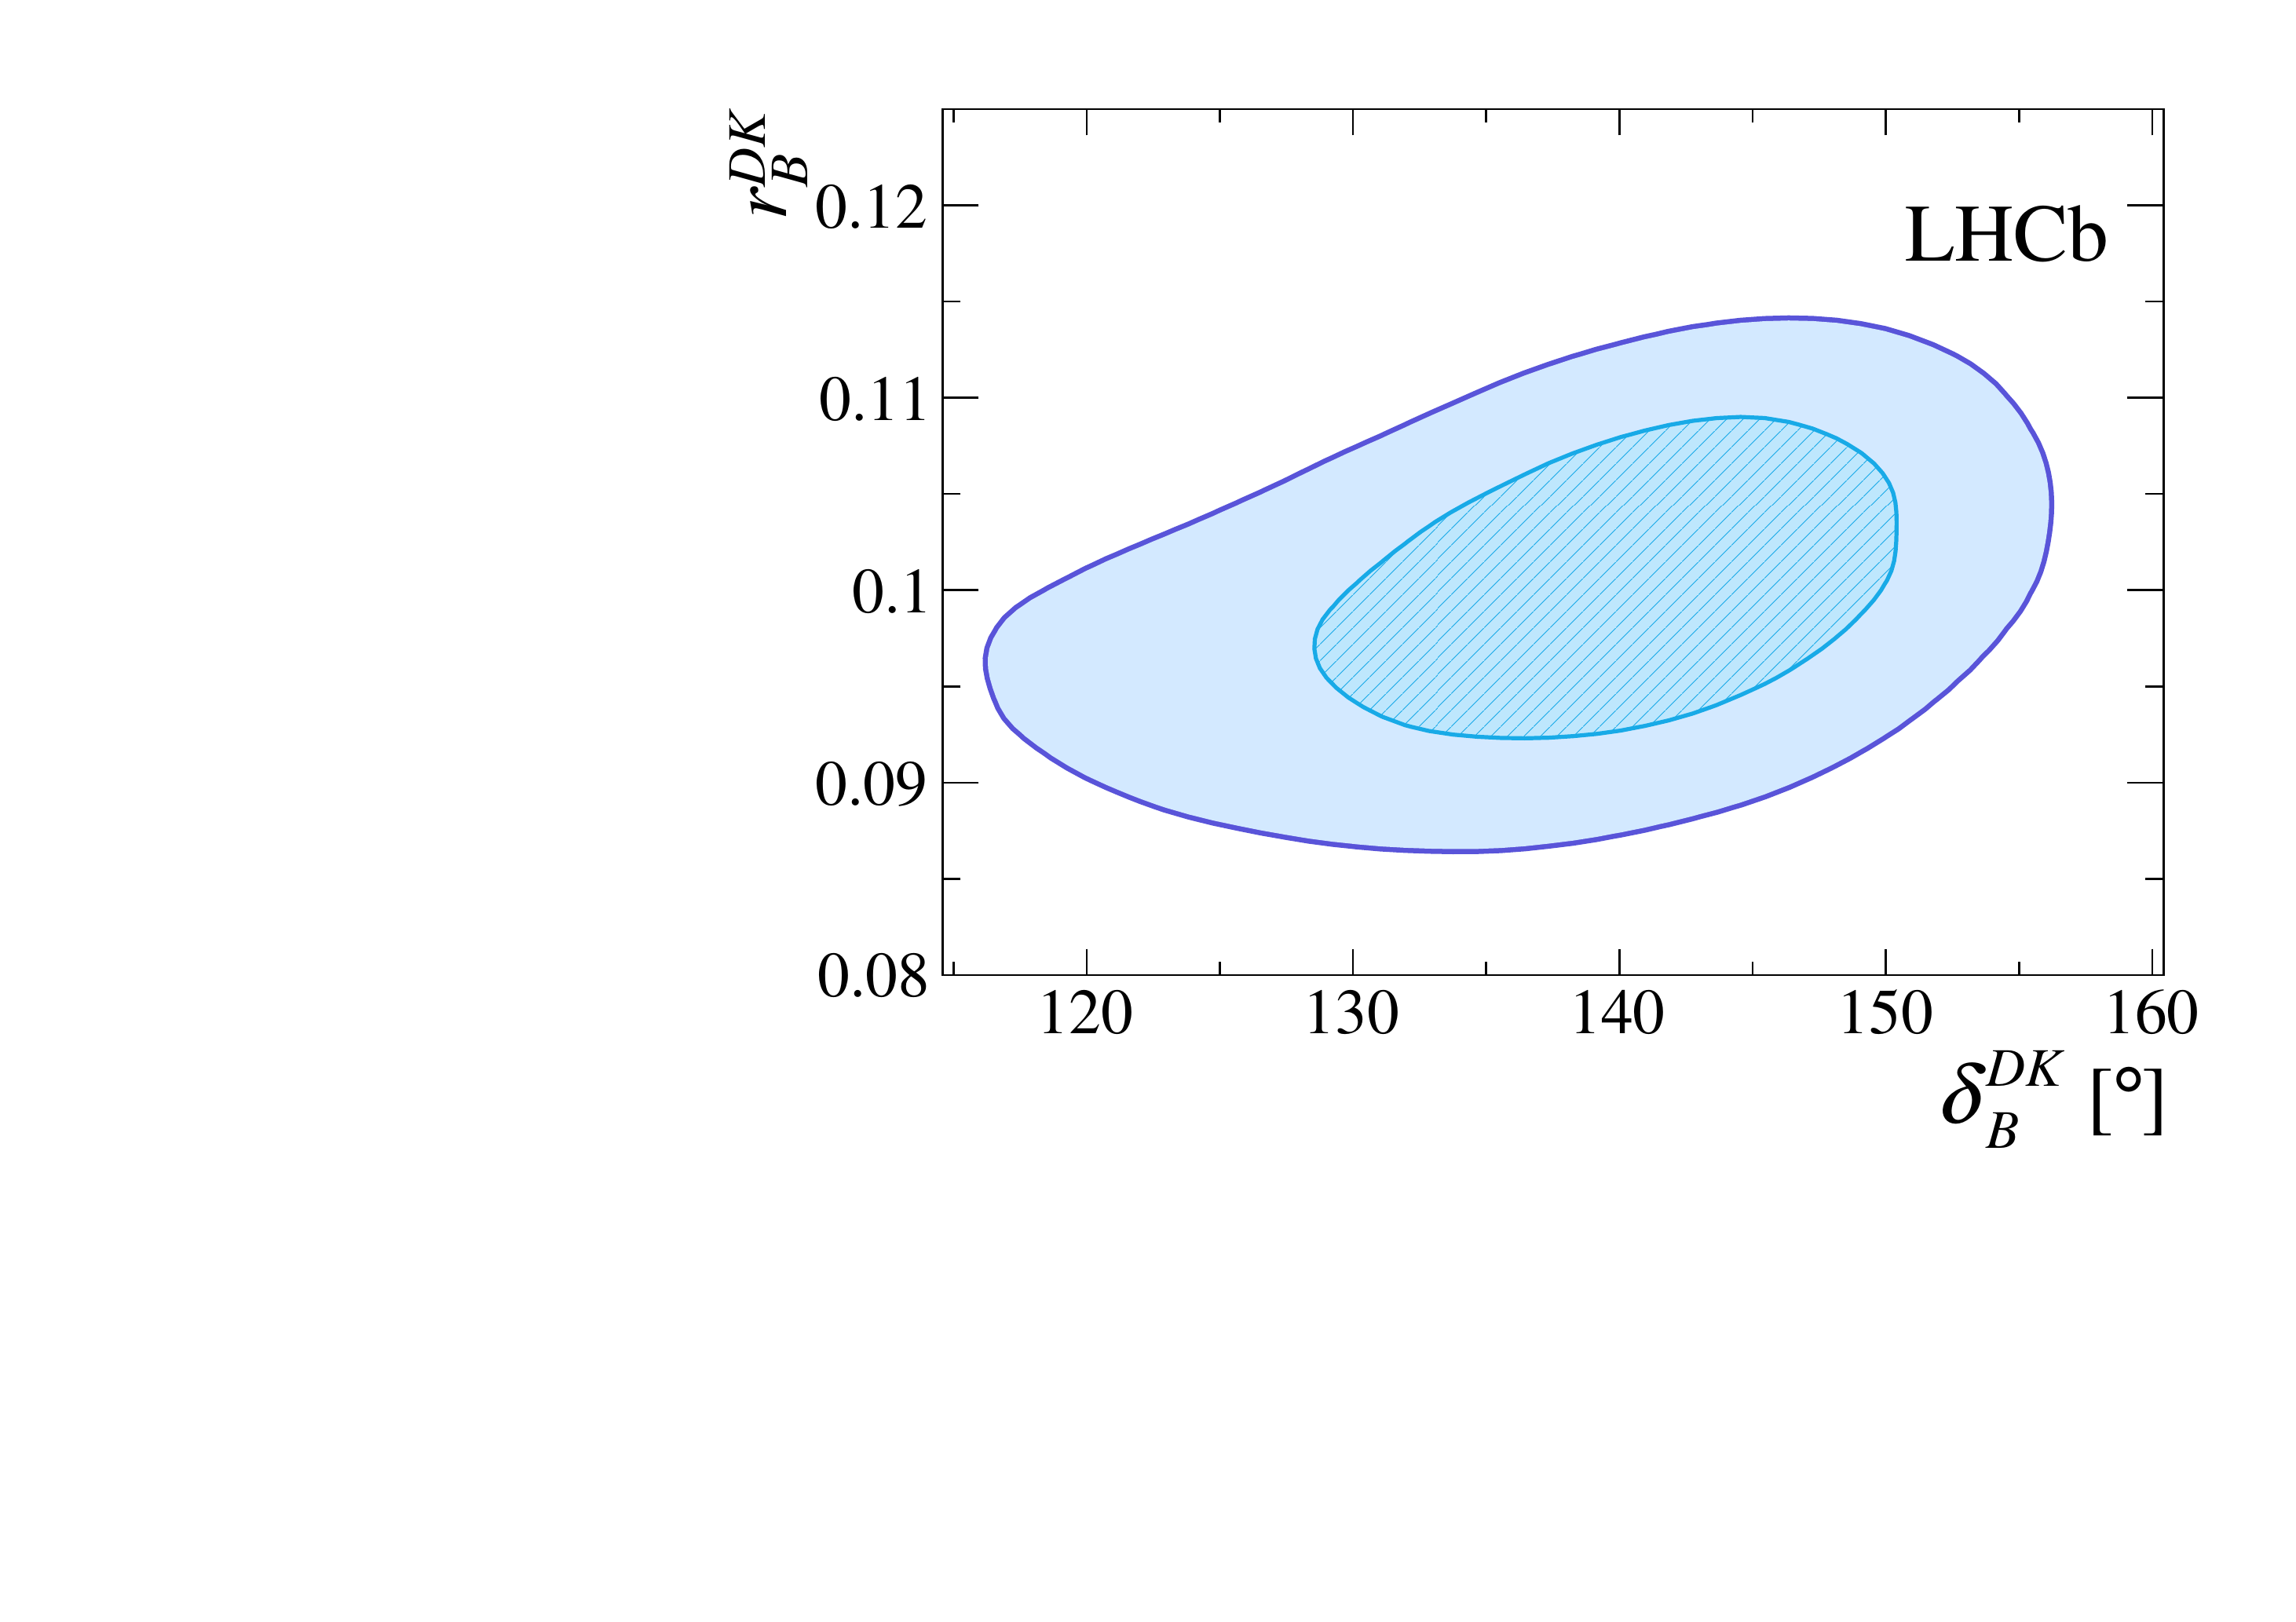}
  \end{center}
  \caption{Profile likelihood contours of \g \vs \db (left) and \g \vs \rb (right) for various \DK sub-combinations: (blue) \BuDK, $\Dz\to h\pi\pi\pi$/$hh^{\prime}\piz$, (pink) \BuDK, $\Dz\to\KS hh$, (light brown) \BuDK, $\Dz\to KK$/$K\pi$/$\pi\pi$, (orange) all \Bu modes and (green) the full combination. Dark and light regions show the intervals containing 68.3\% and 95.5\% respectively.}
  \label{fig:g_d_dk}
\end{figure}

\begin{figure}[h!]
  \begin{center}
    \includegraphics[width=0.48\textwidth]{figs/LHCb-PAPER-2016-032-supplementary/Fig13a.pdf}
    \includegraphics[width=0.48\textwidth]{figs/LHCb-PAPER-2016-032-supplementary/Fig13b.pdf} \\
    \includegraphics[width=0.3\textwidth]{figs/LHCb-PAPER-2016-032-supplementary/Fig13c.pdf}
  \end{center}
  \caption{Profile likelihood contours of \g \vs \dbDKstz (left) and \g \vs \rbDKstz (right) for various \DK sub-combinations: (brown) \BdDKstz, $\Dz\to KK$/$K\pi$/$\pi\pi$, (pink) \BdDKstz, $\Dz\to\KS \pi\pi$, (purple) all \Bd modes and (green) the full combination. Dark and light regions show the intervals containing 68.3\% and 95.5\% respectively.}
  \label{fig:g_d_dkstz}
\end{figure}

%\begin{figure}
    %\centering
    %\includegraphics[width=0.6\textwidth]{figs/LHCb-PAPER-2016-032-supplementary/Fig12.pdf}
    %\caption{Posterior \pdf for the Bayesian \Dh combination}
    %\label{fig:bayes_dh_g}
%\end{figure}

\clearpage
